# Supplementary material for: Unpolarized Quark and Gluon TMD PDFs and FFs at N$^3$LO
Source: arXiv:2012.03256 ancillary file (2020-12-21)
Supplement: Supplementary file 1 [file ancillary_readme.pdf]

# Ancillary Files for “Unpolarized Quark and Gluon TMD PDFs and FFs at N<sup>3</sup>LO”

Ming-xing Luo,<sup>1,\*</sup> Tong-Zhi Yang,<sup>1,†</sup> Hua Xing Zhu,<sup>1,‡</sup> and Yu Jiao Zhu<sup>1,§</sup>

<sup>1</sup>*Zhejiang Institute of Modern Physics, Department of Physics, Zhejiang University, Hangzhou, 310027, China*

In this note we explain the definitions and conventions for the ancillary files associated with the arXiv submission of “Unpolarized Quark and Gluon TMD PDFs and FFs at N<sup>3</sup>LO”.

## TMD BEAM FUNCTION

In the MATHEMATICA file `BeamFunction.m` and `BeamFunctionN.m`, we provide matching coefficients for the transverse-momentum-dependent (TMD) beam function for all partonic channels. They correspond to Eqs. (3.4) in the paper, with

$$\text{Beam}["ji"] = \mathcal{I}_{ji}^{(0)} + \text{as} \mathcal{I}_{ji}^{(1)} + \text{as}^2 \mathcal{I}_{ji}^{(2)} + \text{as}^3 \mathcal{I}_{ji}^{(3)}, \quad (1)$$

where “as” stands for  $\frac{\alpha_s(\mu)}{4\pi}$ ,  $j=q, g$  stands for quark or gluon distributions, and  $i = q, g, q\bar{p}, q\bar{b}, q\bar{b}p$  stands for quark  $q$ , gluon  $g$ , a different flavor of quark  $q'$ , antiquark  $\bar{q}$ , a different flavor of anti-quark  $\bar{q}'$ , respectively. For example, after loading the file, type in `Beam["qqbp"]` will return the result for  $\mathcal{I}_{q\bar{q}'}(x, b_\perp, \mu, \nu)$ .

We use the following definitions and conventions in the file:

$$L_p = L_\perp = \ln(|b_\perp^2| \mu^2 / b_0^2), \quad L_Q = L_Q = 2 \ln(Q/\nu), \quad (2)$$

where  $Q = xP^+$  is the invariant mass of the Drell-Yan lepton pair.

## TMD PARTION DISTRIBUTION FUNCTION

The MATHEMATICA file `TMDPDF.m` and `TMDPDFN.m` give the results for the rapidity-regulator-independent TMD PDFs,

$$f_{\perp,ij}(x, b_\perp, \mu) = \mathcal{I}_{ij}(x, b_\perp, \mu, \nu) \sqrt{\mathcal{S}(b_\perp, \mu, \nu)}. \quad (3)$$

They have the same structure as the file `BeamFunction.m`, with the definition of a new symbol,

$$L_h = L_\nu + L_Q = \ln(Q^2/\mu^2), \quad (4)$$

and

$$\text{TMDpdf}["ji"] = f_{\perp,ji}^{(0)} + \text{as} f_{\perp,ji}^{(1)} + \text{as}^2 f_{\perp,ji}^{(2)} + \text{as}^3 f_{\perp,ji}^{(3)}. \quad (5)$$

When referring to the TMD beam functions and TMD PDFs calculated in this paper, please kindly cite Refs. [3?].

## THE TIME-LIKE TMD COEFFICIENT FUNCTIONS

In the MATHEMATICA file `FFMatchingKernels.m` and `FFMatchingKernelsN.m`, we provide time-like TMD co-

efficient functions for all partonic channels. They correspond to Eqs. (3.6) in the paper, with

$$\text{Frag}["ij"] = \mathcal{C}_{ij}^{(0)} + \text{as} \mathcal{C}_{ij}^{(1)} + \text{as}^2 \mathcal{C}_{ij}^{(2)} + \text{as}^3 \mathcal{C}_{ij}^{(3)}, \quad (6)$$

where  $j=q, g$  stands for quark or gluon fragmentations, and  $i = q, g, q\bar{p}, q\bar{b}, q\bar{b}p$  stands for quark  $q$ , gluon  $g$ , a different flavor of quark  $q'$ , antiquark  $\bar{q}$ , a different flavor of anti-quark  $\bar{q}'$ , respectively. For example, after loading the file, type in `Frag["qbpq"]` will return the result for  $\mathcal{C}_{q\bar{q}'}(z, b_\perp/z, \mu, \nu)$ .

We use the following definitions and conventions in the file:

$$L_p = L_\perp = \ln(|b_\perp^2| \mu^2 / b_0^2), \quad L_Q = L_Q = 2 \ln(Q/\nu), \quad (7)$$

where  $Q = P^+/z$  is twice the energy of the mother parton.

## TMD FRAGMENTATION FUNCTION

The MATHEMATICA file `TMDFF.m` and `TMDFFN.m` give the results for the rapidity-regulator-independent TMDFFs,

$$g_{\perp,ij}(x, b_\perp/z, \mu) = \mathcal{C}_{ij}(x, b_\perp/z, \mu, \nu) \sqrt{\mathcal{S}(b_\perp, \mu, \nu)}. \quad (8)$$

They have the same structure as the file `FFMatchingKernels.m`, with the definition of a new symbol,

$$L_h = L_\nu + L_Q = \ln(Q^2/\mu^2), \quad (9)$$

and

$$\text{TMDFF}["ji"] = g_{\perp,ji}^{(0)} + \text{as} g_{\perp,ji}^{(1)} + \text{as}^2 g_{\perp,ji}^{(2)} + \text{as}^3 g_{\perp,ji}^{(3)}. \quad (10)$$

## RESUMMED TIME-LIKE COEFFICIENT FUNCTIONS

In the MATHEMATICA file `resummedFFsinglets.m`, we provide the Mellin N-space results for the resummed time-like coefficient functions to order  $a_s^{15} = (\alpha_s/(4\pi))^{15}$ , where the expressions of the respective highest three terms in the Laurent expansions about  $\bar{N} = N - 1 = 0$  are given. The corresponding  $z$ -space results are obtained

by inverse Mellin transformation, and according to our definition of the Mellin moments

$$M \left[ \frac{1}{z} \ln^k z \right] \equiv \int_0^1 dz z^{N-1} \frac{1}{z} \ln^k z = \frac{(-1)^k k!}{(N-1)^{k+1}} = \frac{(-1)^k k!}{\overline{N}^{k+1}}, \quad (11)$$

the inversion rule is simply given by

$$\overline{N}^k \rightarrow -\frac{(-1)^{-k}}{(-k-1)!} \ln^{-k-1} z, \quad \forall k < 0. \quad (12)$$

### TMD SOFT FUNCTION

The MATHEMATICA file `softfunction.m` gives the quark TMD soft function to N<sup>3</sup>LO with

$$L_\nu = L_\nu = \ln(\nu^2/\mu^2). \quad (13)$$

Expressions for gluon TMD function is easily obtained by Casimir scaling. The soft zero-bin function is identical to TMD soft function and is universal for both space-like and time-like configurations up to  $\mathcal{O}(\alpha_s^3)$ .

### SYMBOLS AND COLORS

For the color factors,

$$\begin{aligned} \mathbf{CF} &= C_F, \quad \mathbf{Nf} = N_f, \quad \mathbf{TF} = T_F, \quad \mathbf{CA} = C_A, \\ \frac{\mathbf{dabc2}}{\mathbf{nc}} &= \frac{d^{ABC} d_{ABC}}{N_c} = \frac{(N_c^2 - 1)(N_c^2 - 4)}{N_c^2}. \end{aligned} \quad (14)$$

`plusD[n,1-z]` is the conventional plus distribution

$$\text{plusD}[\mathbf{n}, \mathbf{1-z}] = \left( \frac{\ln^n(1-z)}{1-z} \right)_+. \quad (15)$$

Dirac delta function is represented by

$$\mathbf{delta}[\mathbf{1-z}] = \delta(1-z).$$

Harmonic polylogarithms are represented by

$$\mathbf{H}[\mathbf{a1}, \mathbf{a2}, \dots, \mathbf{an}, \mathbf{z}] = \text{HPL}[\{\mathbf{a1}, \mathbf{a2}, \dots, \mathbf{an}\}, \mathbf{z}],$$

and `zeta[n]` is Riemann zeta value  $\zeta_n$ .

When referring to the unpolarized TMD distributions calculated in this paper, please kindly cite Refs. [1–3].

---

\* mingxingluo@zju.edu.cn

† yangtz@zju.edu.cn

‡ zhuhx@zju.edu.cn

§ zhuyujiao@zju.edu.cn

- [1] M.-X. Luo, T.-Z. Yang, H. X. Zhu and Y.J. Zhu, “Unpolarized Quark and Gluon TMD PDFs and FFs at N<sup>3</sup>LO,” [arXiv:2012.xxxxx [hep-ph]].
- [2] M.-X. Luo, T.-Z. Yang, H. X. Zhu and Y.J. Zhu, “Quark Transverse Parton Distribution at the Next-to-Next-to-Next-to-Leading Order,” Phys. Rev. Lett. **124**, no. 9, 092001 (2020) [arXiv:1912.05778 [hep-ph]].
- [3] Y. Li and H. X. Zhu, “Bootstrapping Rapidity Anomalous Dimensions for Transverse-Momentum Resummation,” Phys. Rev. Lett. **118**, no. 2, 022004 (2017) [arXiv:1604.01404 [hep-ph]].
